# Supplementary material for: Investigating the Role of Instruction Variety and Task Difficulty in Robotic Manipulation Tasks
Source: arXiv:2407.03967 source file (2024-10-28)
Supplement: Supplementary file 1 [file para-gdg.tex]

\begin{table*}[tbhp]
\centering
\scriptsize
\sisetup{mode=match,tight-spacing=true,table-format=2.1,table-number-alignment=center}

\setlength{\tabcolsep}{4.5pt}
\begin{tabular}{@{} l *{18}{S} @{}}
\toprule
& {T1} & {T2} & {T3} & {T4} & {T5} & {T6} & {T7} & {T8} & {T9} & {T10} & {T11} & {T12} & {T13} & {T14} & {T15} & {T16} & {T17} & {Avg.} \\
\midrule
\multicolumn{18}{@{}l}{\textit{\textbf{Noop}}} \\
\addlinespace[1pt]
L1 &99.5 & 100.0 & 99.5 & 98.5 & 62.5 & 100.0 & 100.0 & {---} & 11.5 & {---} & 92.0 & 97.5 & {---} & {---} & 99.0 & 43.5 & 72.0 & 82.7 \\
L2 &99.0 & 100.0 & 99.5 & 98.0 & 55.5 & 100.0 & 100.0 & {---} & 13.5 & {---} & 91.5 & 92.5 & {---} & {---} & 97.0 & 48.0 & 69.0 & 81.8 \\
L3 &99.0 & 99.0 & 99.5 & 99.0 & 68.5 & 99.0 & 99.0 & {---} & 15.5 & {---} & 93.0 & {---} & {---} & {---} & 99.0 & 48.5 & 10.0 & 77.4 \\
L4 &{---} & {---} & {---} & {---} & {---} & {---} & {---} & 93.0 & {---} & 0.5 & {---} & {---} & 0.0 & 98.5 & {---} & {---} & {---} & 48.0 \\
\midrule[0.5pt]
\multicolumn{18}{@{}l}{\textit{\textbf{Perturbed with Gobbledygook Tokens}}} \\
\addlinespace[1pt]
L1 &89.5 & 74.5 & 5.5 & 73.5 & 8.5 & 92.5 & 90.0 & {---} & 1.0 & {---} & 92.5 & 94.0 & {---} & {---} & 29.0 & 19.5 & 67.5 & 56.7 \\
L2 &89.5 & 67.5 & 5.0 & 71.5 & 12.0 & 86.5 & 89.5 & {---} & 0.5 & {---} & 92.0 & 93.5 & {---} & {---} & 25.0 & 19.0 & 56.5 & 54.5 \\
L3 &63.0 & 48.0 & 7.5 & 75.0 & 11.5 & 59.5 & 59.5 & {---} & 0.0 & {---} & 93.5 & {---} & {---} & {---} & 10.5 & 11.0 & 0.5 & 36.6 \\
L4 &{---} & {---} & {---} & {---} & {---} & {---} & {---} & 72.5 & {---} & 0.0 & {---} & {---} & 0.0 & 19.0 & {---} & {---} & {---} & 22.9 \\
\midrule[0.5pt]
\multicolumn{18}{@{}l}{\textit{\textbf{Perturbed with Gobbledygook Words}}} \\
\addlinespace[1pt]
L1 &95.0 & 98.5 & 9.5 & 17.0 & 4.5 & 98.0 & 99.5 & {---} & 0.5 & {---} & 56.0 & 90.5 & {---} & {---} & 58.5 & 17.0 & 16.5 & 50.8 \\
L2 &95.5 & 97.0 & 7.0 & 23.0 & 2.5 & 99.0 & 100.0 & {---} & 1.5 & {---} & 52.5 & 93.0 & {---} & {---} & 64.5 & 25.0 & 13.5 & 51.8\\
L3 &74.5 & 86.5 & 6.0 & 23.5 & 3.0 & 93.5 & 87.5 & {---} & 0.0 & {---} & 56.5 & {---} & {---} & {---} & 37.0 & 11.0 & 0.0 & 39.9\\
L4 &{---} & {---} & {---} & {---} & {---} & {---} & {---} & 85.5 & {---} & 0.0 & {---} & {---} & 0.0 & 49.5 & {---} & {---} & {---} & 33.8\\
\bottomrule
\end{tabular}
\caption{Effects of training on paraphrases through evaluations of either no further perturbations, Gobbledygook Tokens, or Gobbledygook Words. The leftmost column denotes increasing difficulty levels of generalisation per task ranging from L1 to L4. The topmost row explains results of each training/evaluation split across all 17 different tasks. L4 generalisation difficulty only exists in some tasks.}
\label{tab:full-paraphrase-gdg-results}
\end{table*}
