# Supplementary material for: Investigating the Role of Instruction Variety and Task Difficulty in Robotic Manipulation Tasks
Source: arXiv:2407.03967 source file (2024-10-28)
Supplement: Supplementary file 3 [file perf-default-full.tex]

% On original instructions
\begin{table*}[tbh]
\centering
\scriptsize
\sisetup{table-format=2.1}

\setlength{\tabcolsep}{4.5pt}
\begin{tabular}{@{} l *{18}{S} @{}}
\toprule
& {T1} & {T2} & {T3} & {T4} & {T5} & {T6} & {T7} & {T8} & {T9} & {T10} & {T11} & {T12} & {T13} & {T14} & {T15} & {T16} & {T17} & {Avg.} \\
\midrule
\multicolumn{18}{@{}l}{\textit{\textbf{Cross-attention + Obj-Centric}}} \\
\addlinespace[1pt]
\bfseries L1 & 100.0 & 99.5 & 99.5 & 97.0 & 8.5 & 100.0 & 100.0 & {---} & 19.0 & {---} & 91.5 & 96.0 & {---} & {---} & 96.5 & 49.5 & 73.5 & 79.3 \\
\bfseries L2 & 99.5 & 99.5 & 100.0 & 98.0 & 9.5 & 99.0 & 99.5 & {---} & 18.0 & {---} & 95.0 & 96.5 & {---} & {---} & 92.0 & 47.5 & 71.0 & 78.8 \\
\bfseries L3 & 100.0 & 99.0 & 100.0 & 99.0 & 10.0 & 98.5 & 99.5 & {---} & 14.0 & {---} & 90.5 & {---} & {---} & {---} & 93.0 & 43.0 & 21.5 & 72.3 \\
\bfseries L4 & {---} & {---} & {---} & {---} & {---} & {---} & {---} & 96.5 & {---} & 0.5 & {---} & {---} & 0.0 & 97.5 & {---} & {---} & {---} & 48.6 \\
\multicolumn{18}{@{}l}{\textit{\textbf{Cross-attention + Patches}}} \\
\addlinespace[1pt]
\bfseries L1 & 91.5 & 75.0 & 97.5 & 12.0 & 1.0 & 76.5 & 95.0 & {---} & 9.0 & {---} & 90.5 & 93.0 & {---} & {---} & 79.5 & 95.5 & 2.5 & 63.0 \\
\bfseries L2 & 94.0 & 73.5 & 96.5 & 9.5 & 2.5 & 78.5 & 92.0 & {---} & 14.0 & {---} & 87.5 & 91.5 & {---} & {---} & 71.5 & 94.5 & 0.0 & 62.0 \\
\bfseries L3 & 57.0 & 70.0 & 68.0 & 9.0 & 0.5 & 72.5 & 57.5 & {---} & 11.5 & {---} & 85.0 & {---} & {---} & {---} & 62.0 & 44.0 & 2.0 & 44.9 \\
\bfseries L4 & {---} & {---} & {---} & {---} & {---} & {---} & {---} & 25.5 & {---} & 1.0 & {---} & {---} & 0.0 & 29.0 & {---} & {---} & {---} & 13.9 \\
% \midrule[0.3pt]
\multicolumn{18}{@{}l}{\textit{\textbf{Concatenate + Obj-Centric}}} \\
\addlinespace[1pt]
\bfseries L1 & 100.0 & 100.0 & 99.5 & 97.0 & 19.0 & 100.0 & 100.0 & {---} & 13.5 & {---} & 88.5 & 95.0 & {---} & {---} & 96.0 & 45.5 & 75.5 & 79.2 \\
\bfseries L2 & 99.5 & 100.0 & 99.5 & 99.0 & 19.0 & 100.0 & 100.0 & {---} & 16.0 & {---} & 91.0 & 95.5 & {---} & {---} & 92.0 & 39.0 & 74.5 & 78.8 \\
\bfseries L3 & 98.0 & 97.0 & 100.0 & 99.0 & 21.0 & 92.0 & 96.5 & {---} & 18.5 & {---} & 95.0 & {---} & {---} & {---} & 96.5 & 43.0 & 68.5 & 77.1 \\
\bfseries L4 & {---} & {---} & {---} & {---} & {---} & {---} & {---} & 97.0 & {---} & 2.5 & {---} & {---} & 0.0 & 97.5 & {---} & {---} & {---} & 49.2 \\
\multicolumn{18}{@{}l}{\textit{\textbf{Concatenate + Patches}}} \\
\bfseries L1 & 96.0 & 84.5 & 97.5 & 13.0 & 2.5 & 87.0 & 95.0 & {---} & 42.5 & {---} & 96.0 & 96.5 & {---} & {---} & 75.0 & 94.0 & 4.0 & 68.0 \\
\bfseries L2 & 92.5 & 73.5 & 97.5 & 17.0 & 3.5 & 93.5 & 91.0 & {---} & 31.0 & {---} & 95.5 & 88.0 & {---} & {---} & 75.0 & 96.5 & 7.0 & 66.3 \\
\bfseries L3 & 71.5 & 66.5 & 91.0 & 12.5 & 3.5 & 93.0 & 58.0 & {---} & 30.5 & {---} & 87.0 & {---} & {---} & {---} & 58.5 & 61.0 & 2.0 & 52.9 \\
\bfseries L4 & {---} & {---} & {---} & {---} & {---} & {---} & {---} & 44.0 & {---} & 11.0 & {---} & {---} & 0.0 & 38.5 & {---} & {---} & {---} & 23.4 \\
\addlinespace[1pt]
\bottomrule
\end{tabular}
\caption{perf default full}
\label{tab:perf-default-full}
\end{table*}
