# Supplementary material for: Investigating the Role of Instruction Variety and Task Difficulty in Robotic Manipulation Tasks
Source: arXiv:2407.03967 source file (2024-10-28)
Supplement: Supplementary file 4 [file perf-default.tex]

% trained on paraphrases
% \begin{table}[tb]
% \centering
% \footnotesize
% \sisetup{table-format=2.1}
% \renewcommand{\arraystretch}{1.3}
% \begin{tabularx}{\linewidth}{@{} X SSSS @{}}
% \toprule
% & {L1} & {L2} & {L3} & {L4} \\
% \midrule
% Cross-Attn + Obj-Centric & \bfseries 82.7 & \bfseries 81.8 & \bfseries 77.4 & \uline{48.0} \\
% Cross-Attn + Patches & 65.0 & 62.6 & 49.5 & 19.5 \\
% Concatenate + Obj-Centric  & \uline{79.5} & \uline{79.3} & \uline{75.9} & \bfseries 49.8 \\
% Concatenate + Patches & 67.9 & 64.4 & 51.5 & 21.8 \\
% \bottomrule
% \end{tabularx}
% \caption{Performance per level for all models without any perturbations. Per-task results are in \cref{tab:perf-default-full}.}
% \label{tab:perf-default}
% \end{table}

% trained on original
\begin{table}[tb]
\centering
\footnotesize
\sisetup{table-format=2.1}

\begin{tabularx}{\linewidth}{@{} X SSSS @{}}
\toprule
& {L1} & {L2} & {L3} & {L4} \\
\midrule
Cross-Attn + Obj-Centric & \bfseries 79.3 & \bfseries 78.8 & \uline{72.3} & \uline{48.6} \\
Cross-Attn + Patches & 63.0 & 62.0 & 44.9 & 13.9 \\
Concatenate + Obj-Centric  & \bfseries 79.2 & \bfseries 78.8 & \bfseries 77.1 & \bfseries 49.2 \\
Concatenate + Patches & 68.0 & 66.3 & 52.9 & 23.4 \\
\bottomrule
\end{tabularx}
\caption{Performance per level for all models without any perturbations. Per-task results are in \cref{tab:perf-default-full}.}
\label{tab:perf-default}
\end{table}
